# Supplementary material for: DriveGPT4: Interpretable End-to-end Autonomous Driving via Large Language Model
Source: arXiv:2310.01412 source file (2024-11-09)
Supplement: Supplementary file 1 [file fig_gpt4_v_appendix.tex]

\begin{figure}[!h]
  \centering
    \includegraphics[width=0.89\linewidth]{imgs/gpt4-v-2.pdf}
     \vspace{-5pt}
  \caption{Comparison between GPT4-V and DriveGPT4. In this example, GPT-V fails to correctly identify the dynamics of the vehicle and cannot generate numerical control signal predictions.}
  \label{gpt4-v_example_2}
\vspace{-5pt}
\end{figure}

\begin{figure}[!h]
  \centering
    \includegraphics[width=0.89\linewidth]{imgs/gpt4-v-3.pdf}
     \vspace{-5pt}
  \caption{Comparison between GPT4-V and DriveGPT4. In this example, GPT-V fails to generate numerical control signal predictions.}
  \label{gpt4-v_example_3}
\vspace{-5pt}
\end{figure}

\begin{figure}[!h]
  \centering    \includegraphics[width=0.89\linewidth]{imgs/gpt4-v-4.pdf}
     \vspace{-5pt}
  \caption{Comparison between GPT4-V and DriveGPT4. In this example, GPT-V cannot generate numerical control signal predictions.}
  \label{gpt4-v_example_4}
\vspace{-5pt}
\end{figure}
